# Supplementary material for: AP-BSN: Self-Supervised Denoising for Real-World Images via Asymmetric PD and Blind-Spot Network
Source: arXiv:2203.11799 source file (2022-03-24)
Supplement: Supplementary file 1 [file fig_network.tex]

\begin{figure*}[t!]
    \renewcommand{\wp}{1.0\linewidth}
    \centering
    \includegraphics[width=\wp]{_src/supple/network/network.pdf}
    \\
    \vspace{-2mm}
    \caption{
        \textbf{Visualization of BSN architecture in our \proposed{}.}
        We modify the network D-BSN from Wu~\etal~\cite{DBSN} into the network have more layer channel, basic modules.
        Also instead of using Multiple Dialted Convolution (MDC) module, our BSN utilizes Dilated Convolution (DC) module which has single branch of dilated convolution layer.
        More details about D-BSN are available in Wu~\etal~\cite{DBSN}.
    }
    \label{fig:network}
    \vspace{-4mm}
\end{figure*}
