# Supplementary material for: AP-BSN: Self-Supervised Denoising for Real-World Images via Asymmetric PD and Blind-Spot Network
Source: arXiv:2203.11799 source file (2022-03-24)
Supplement: Supplementary file 2 [file tab_network.tex]

\begin{table}[t]
    \centering
    \definecolor{Gray}{gray}{0.95}
    \begin{tabularx}{\linewidth}{cc >{\centering\arraybackslash}X >{\centering\arraybackslash}X | cc}
        \toprule
        %\makecell{w/o RPR \\ \footnotesize{PSNR (dB)}}
        \makecell{BSN} & \makecell{layer \\ channel} & module & params & PSNR$^\uparrow$(dB) \\
        \midrule
        \makecell{modified \\ (used)} & 128 & 9 DC & 3.7M & ??.?? \\
        D-BSN & 96 & 6 MDC & 4.0M & ??.?? \\
        \bottomrule
    \end{tabularx}
    \caption{
        \textbf{Ablation study on BSN architecture on SIDD validation dataset.}
        First row box
    }
    \label{tab:network}
\end{table}
